# Supplementary material for: Differentiable Inverse Rendering with Interpretable Basis BRDFs
Source: arXiv:2411.17994 source file (2024-12-01)
Supplement: Supplementary file 2 [file synthetic_supp.pdf]

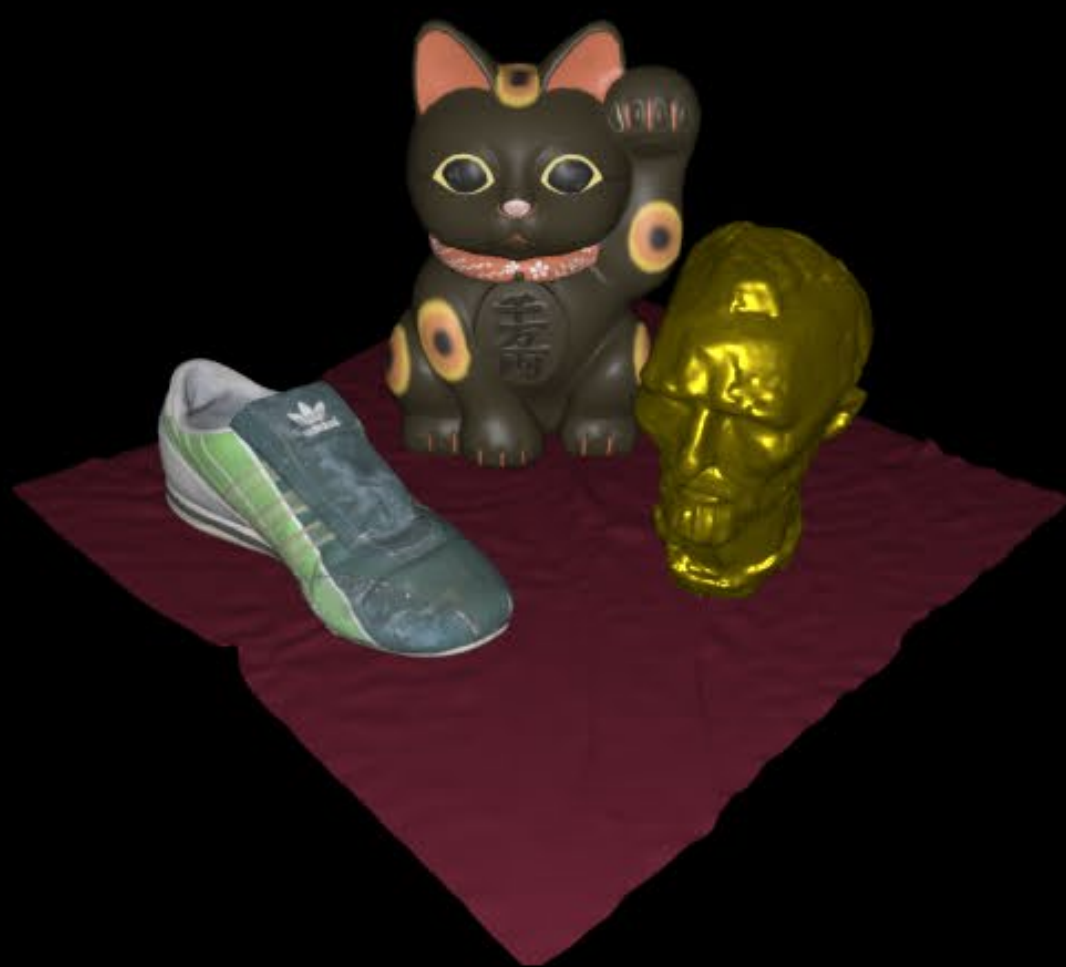

GT

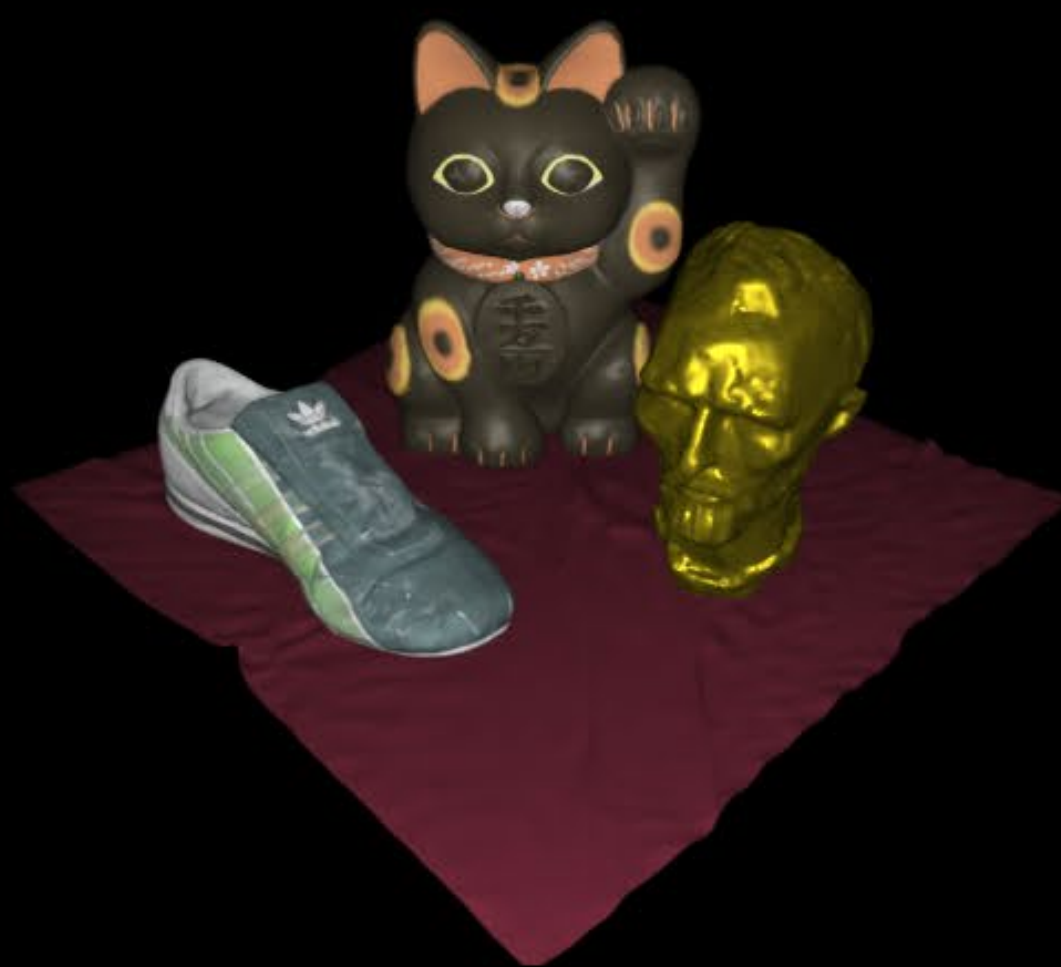

Rendered image

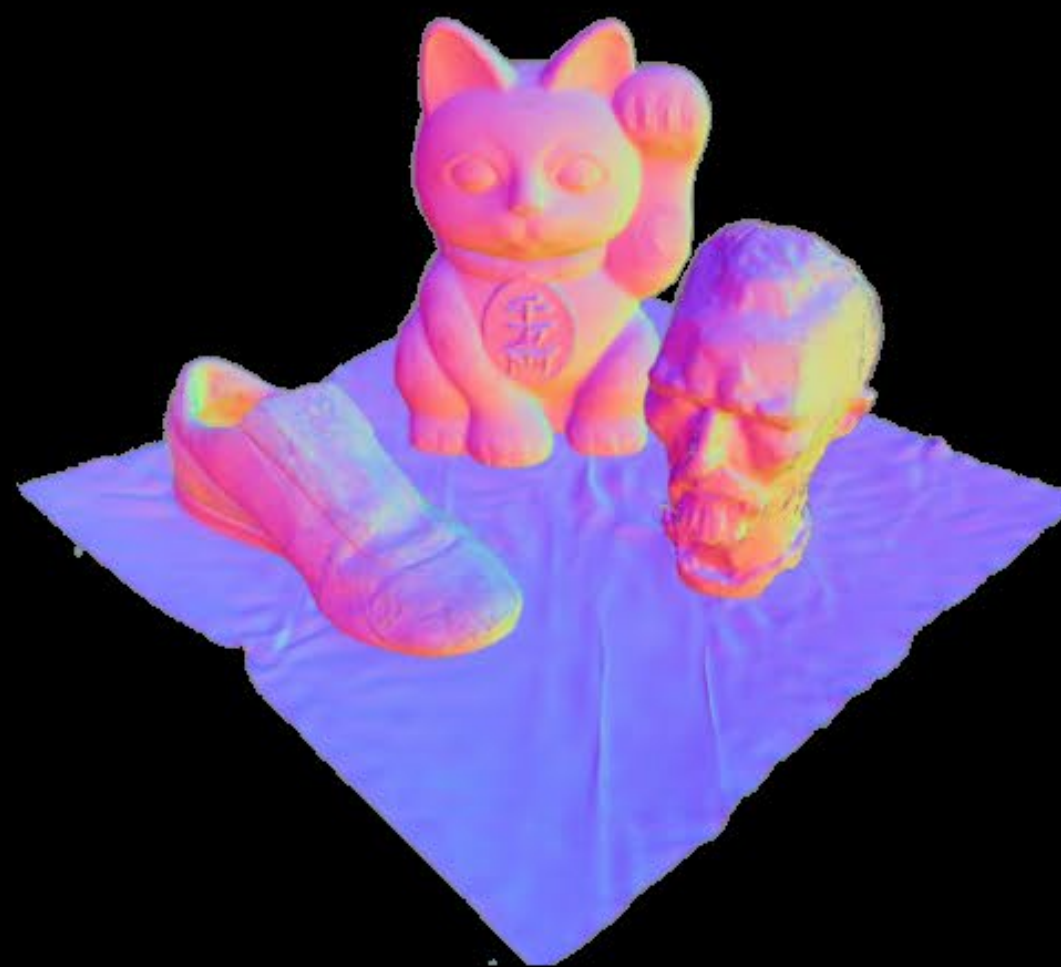

Normal

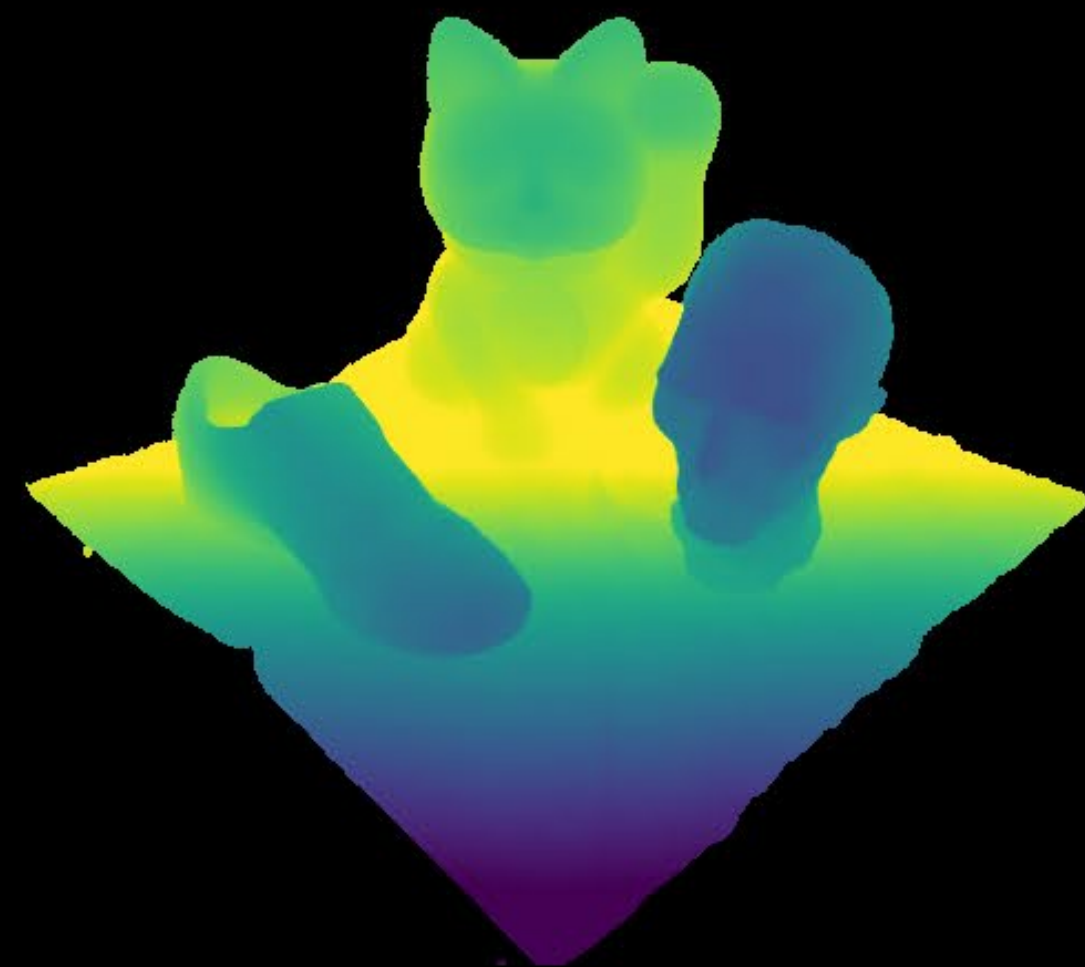

Depth

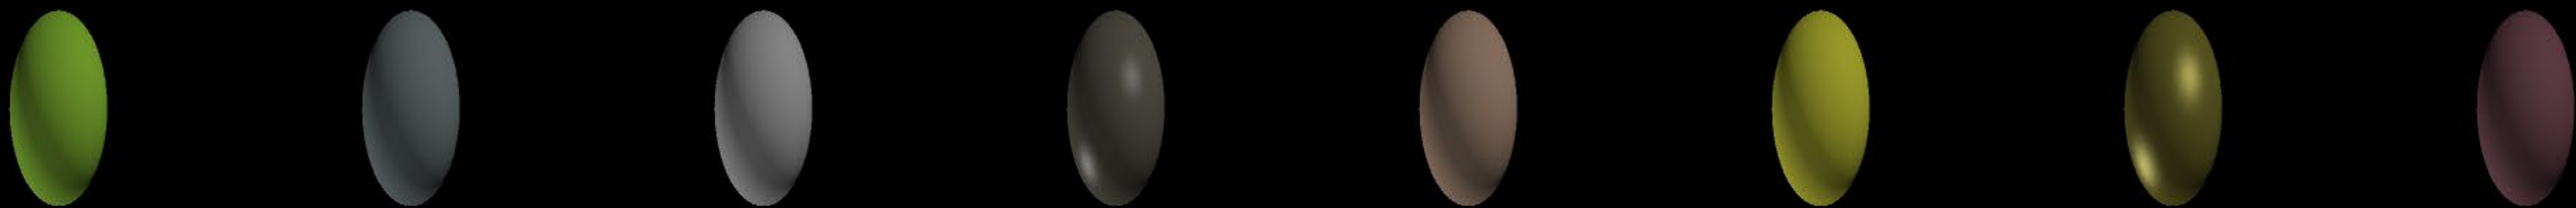

Basis BRDFs

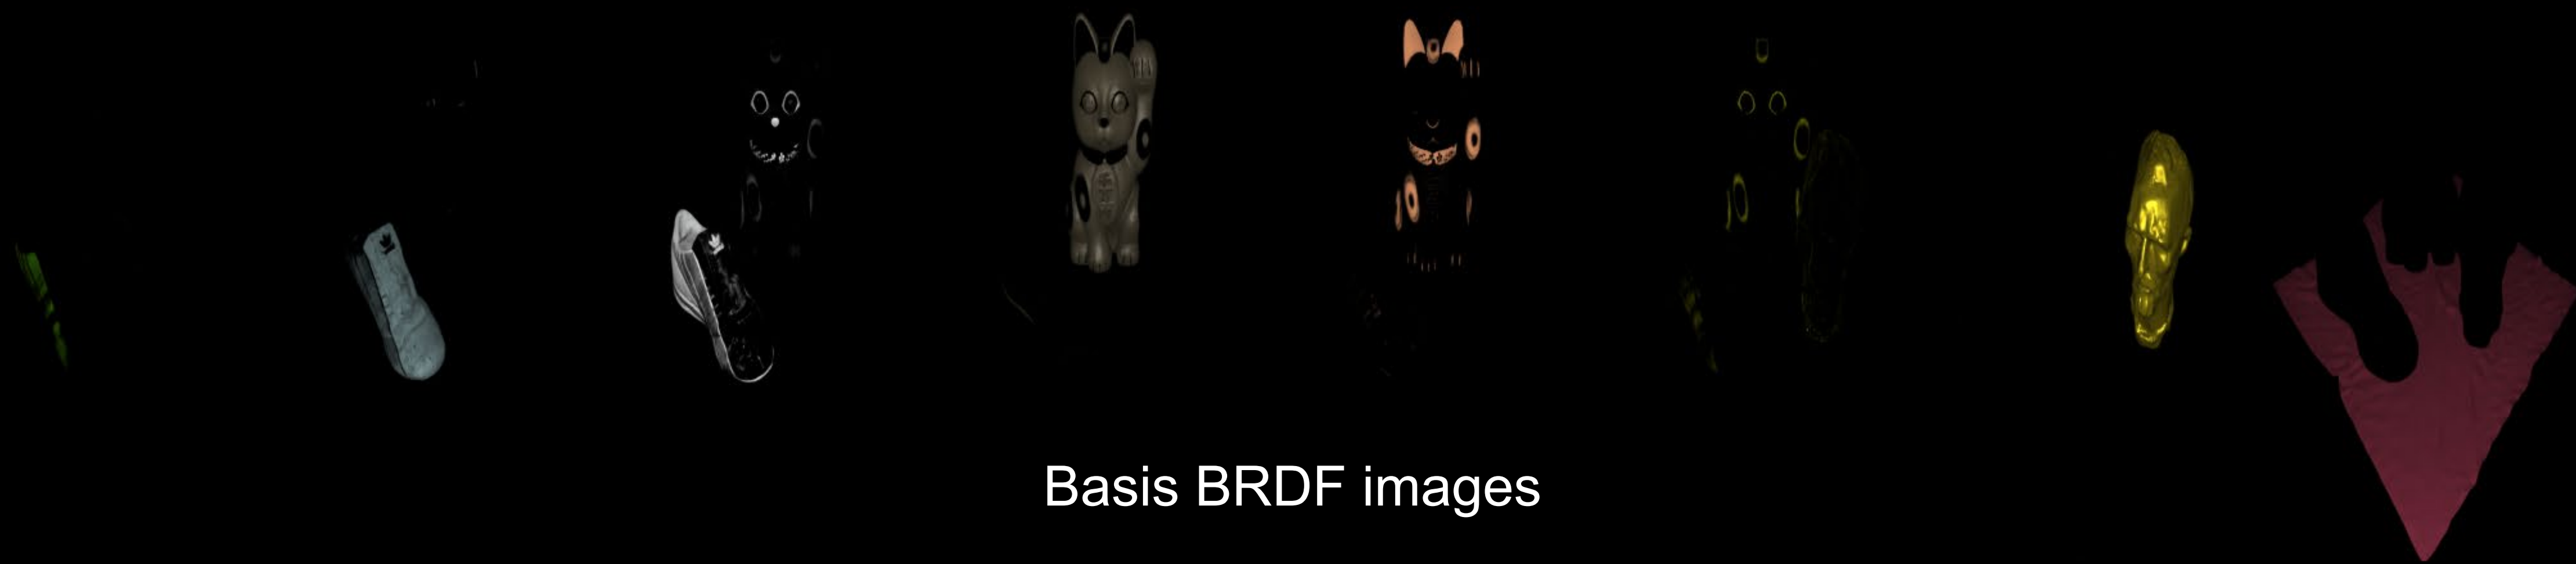

Basis BRDF images

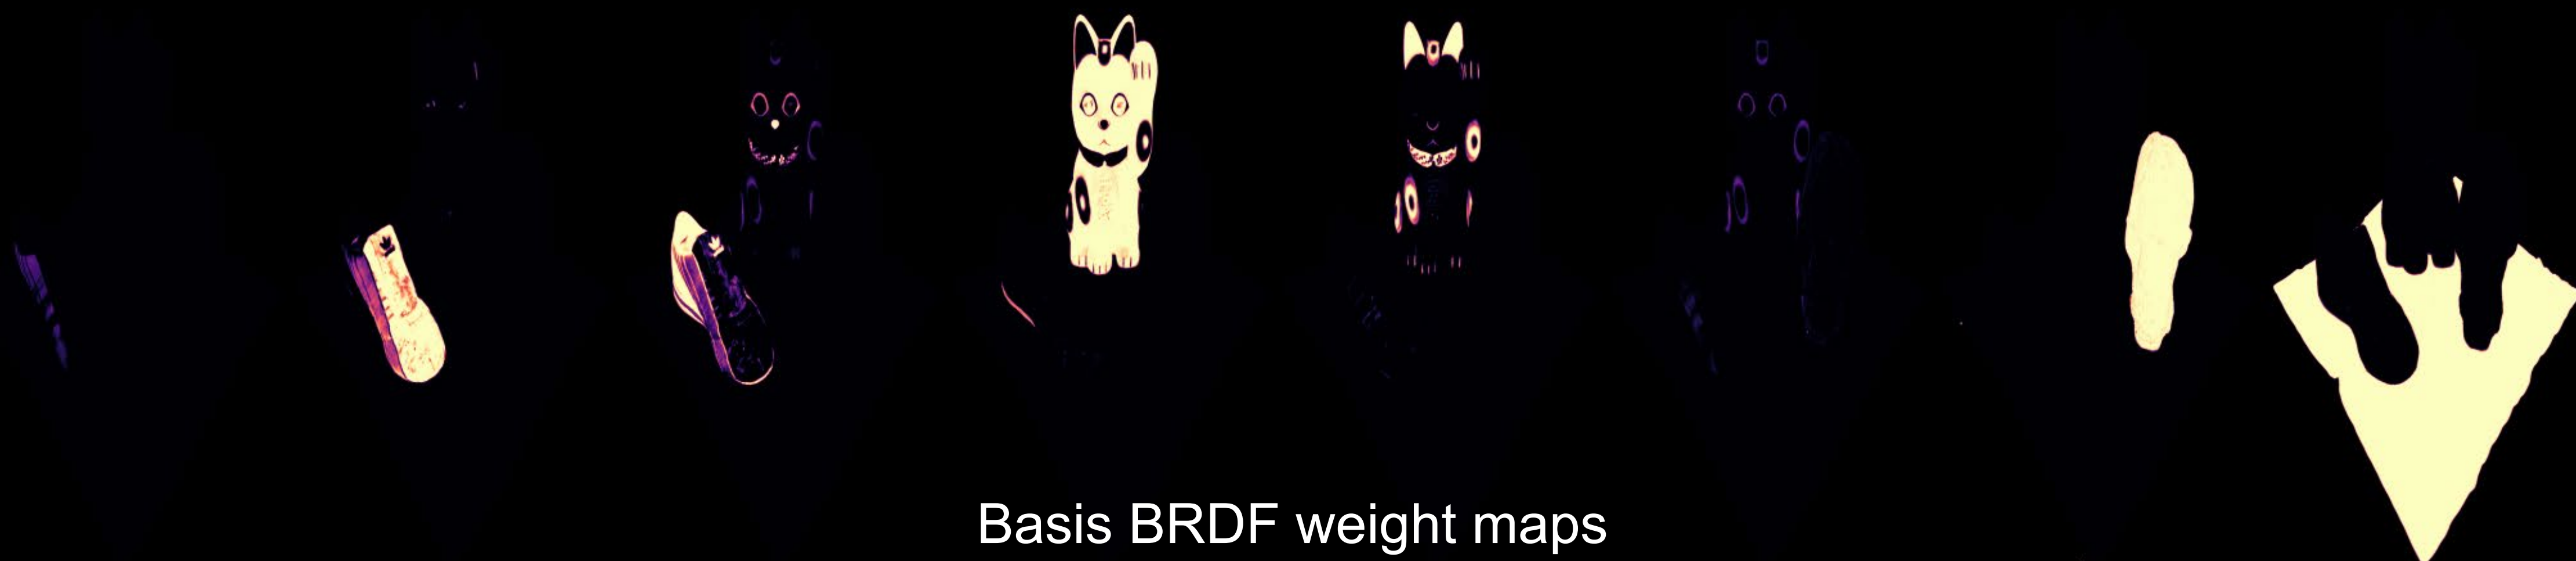

Basis BRDF weight maps



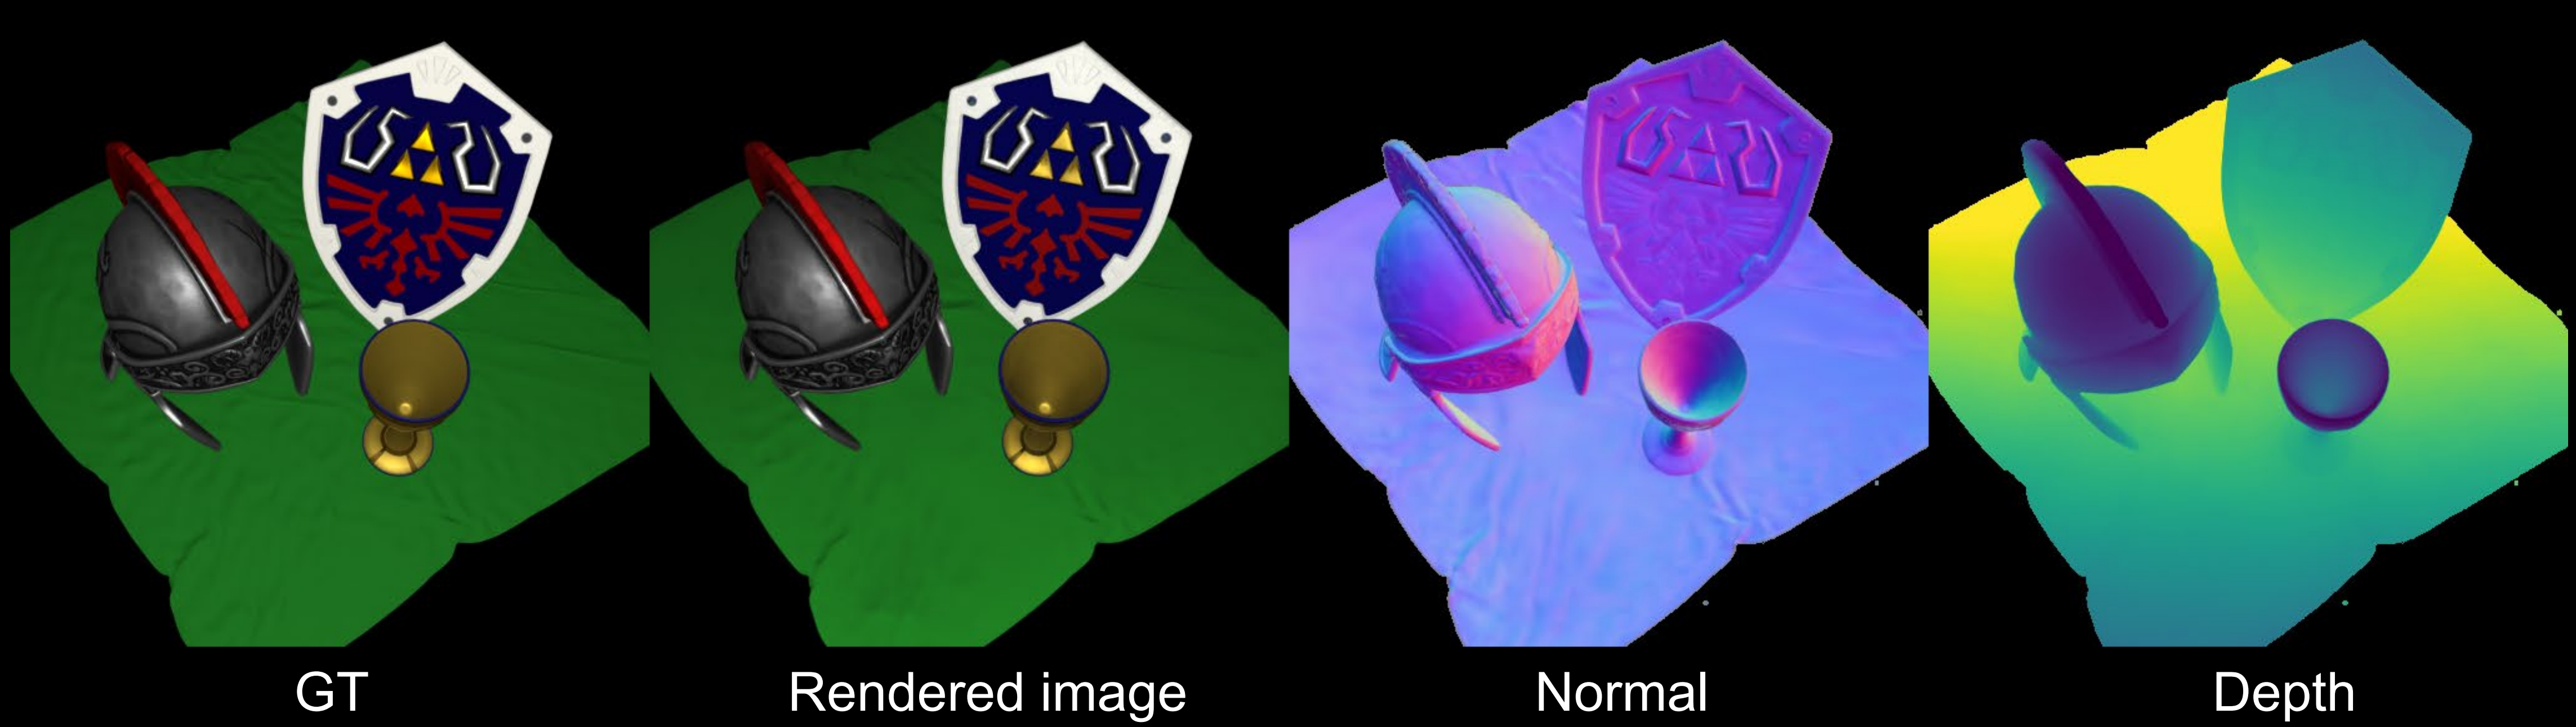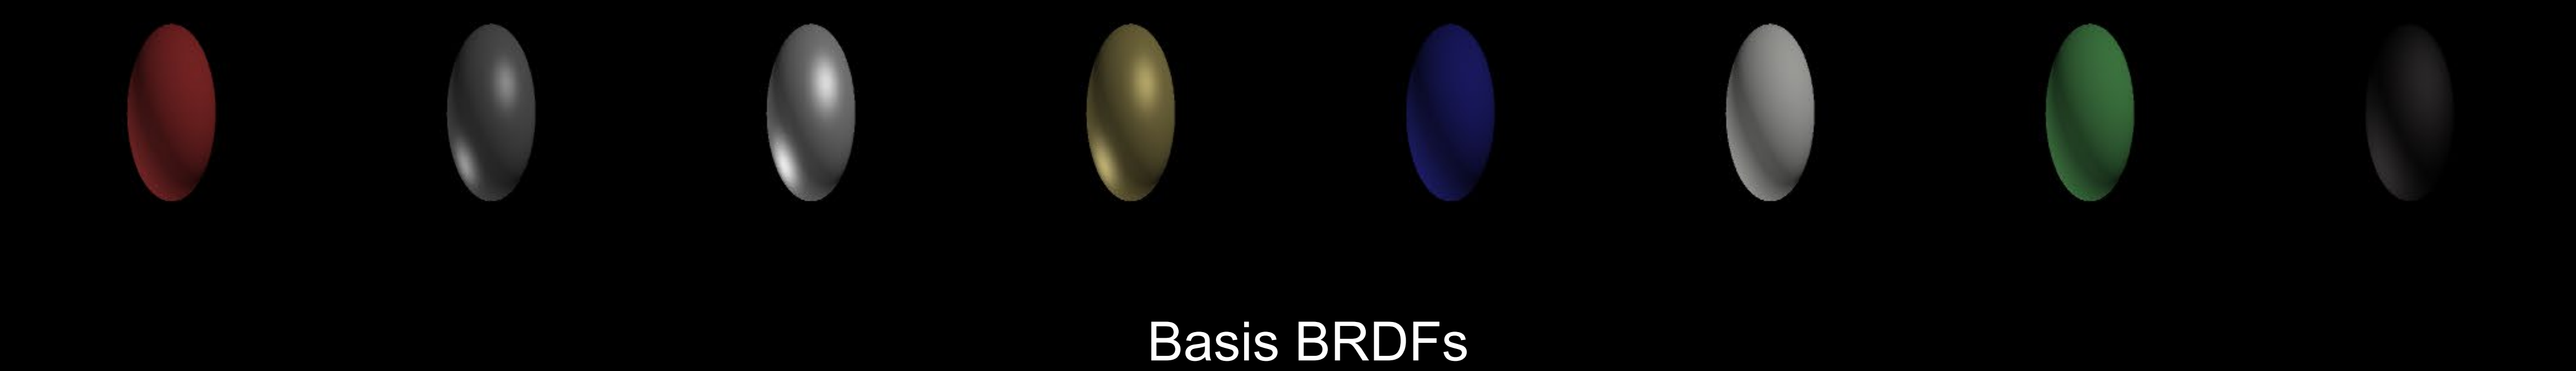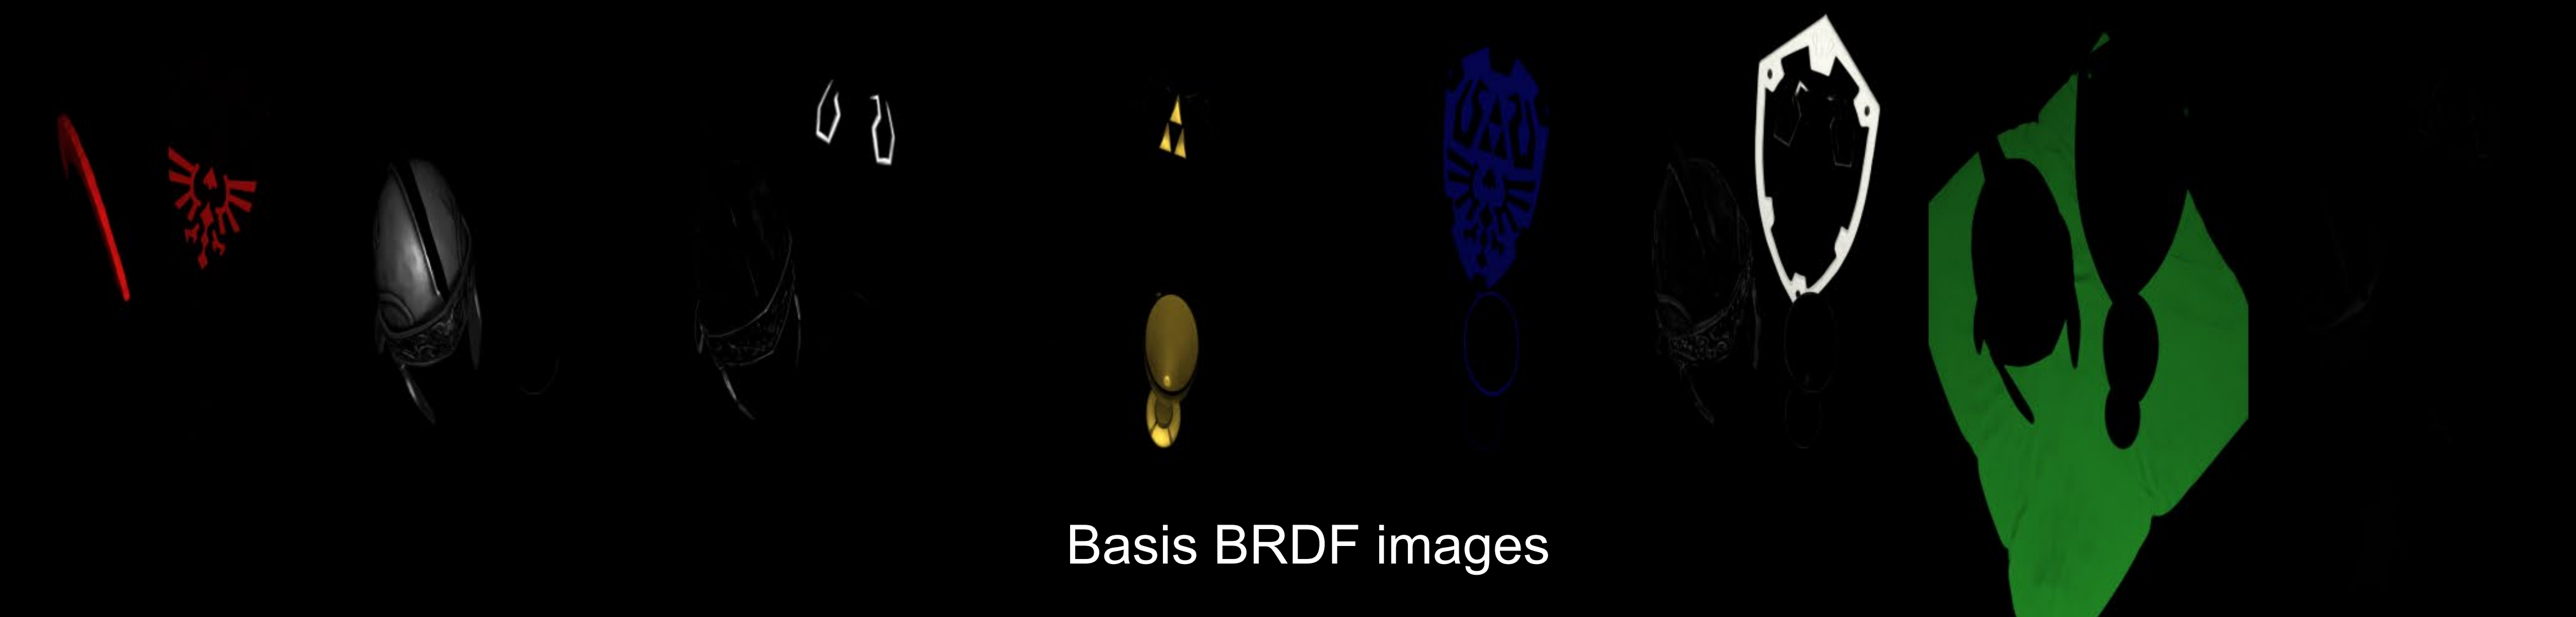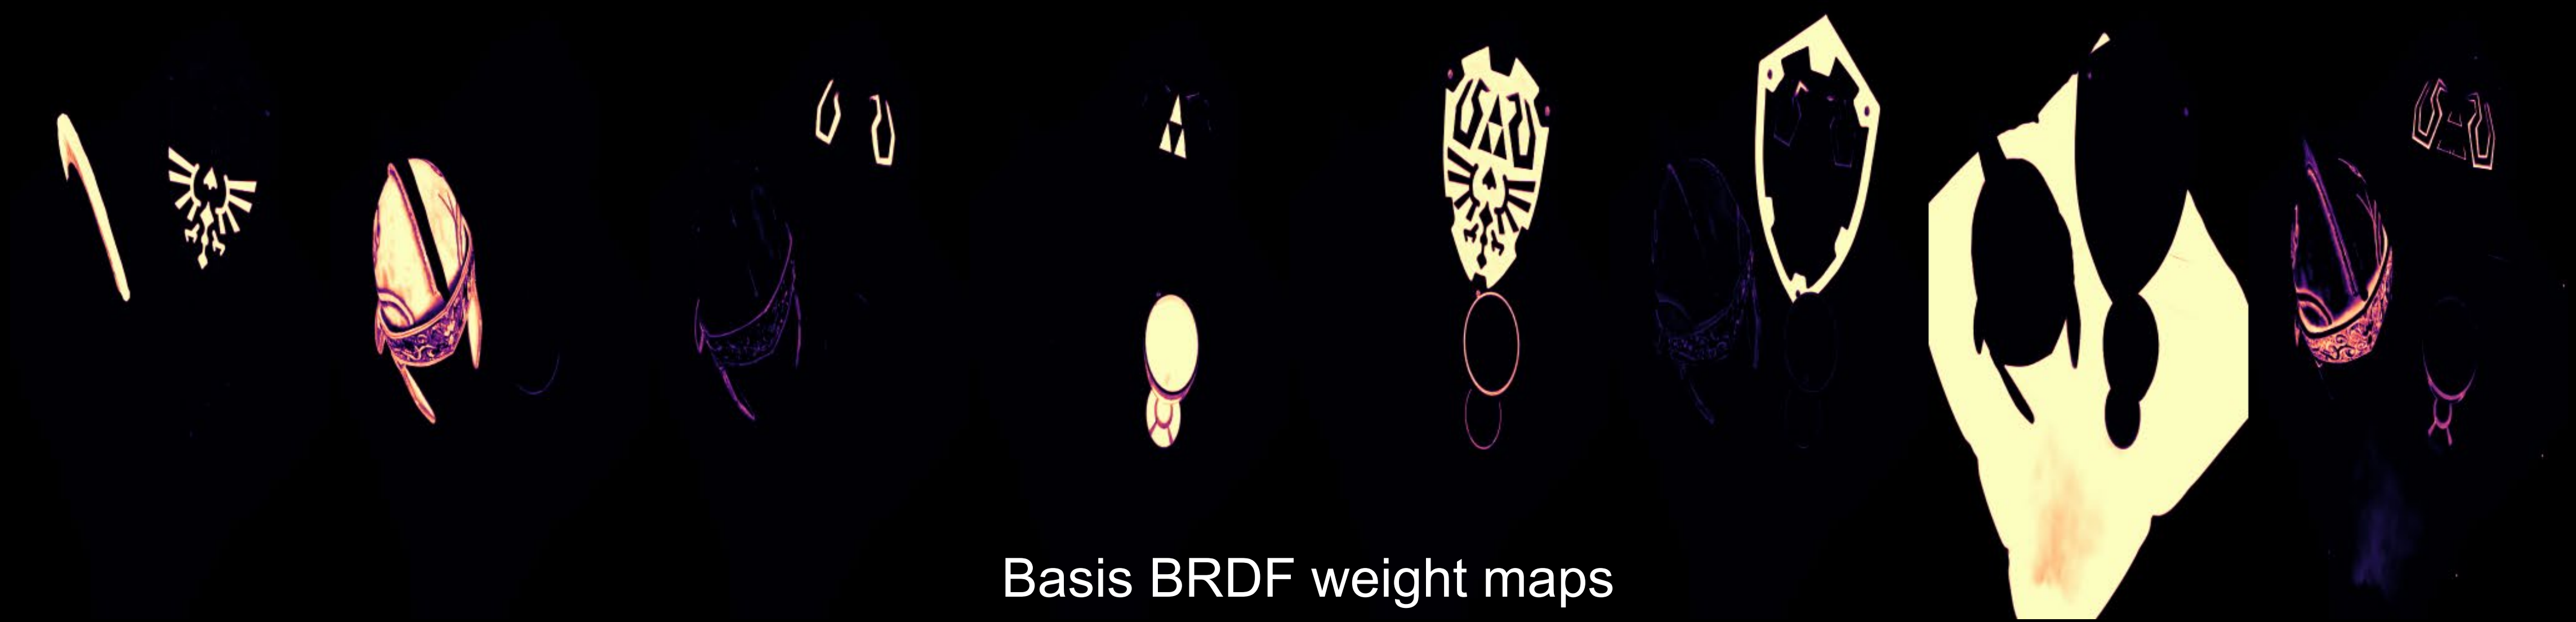



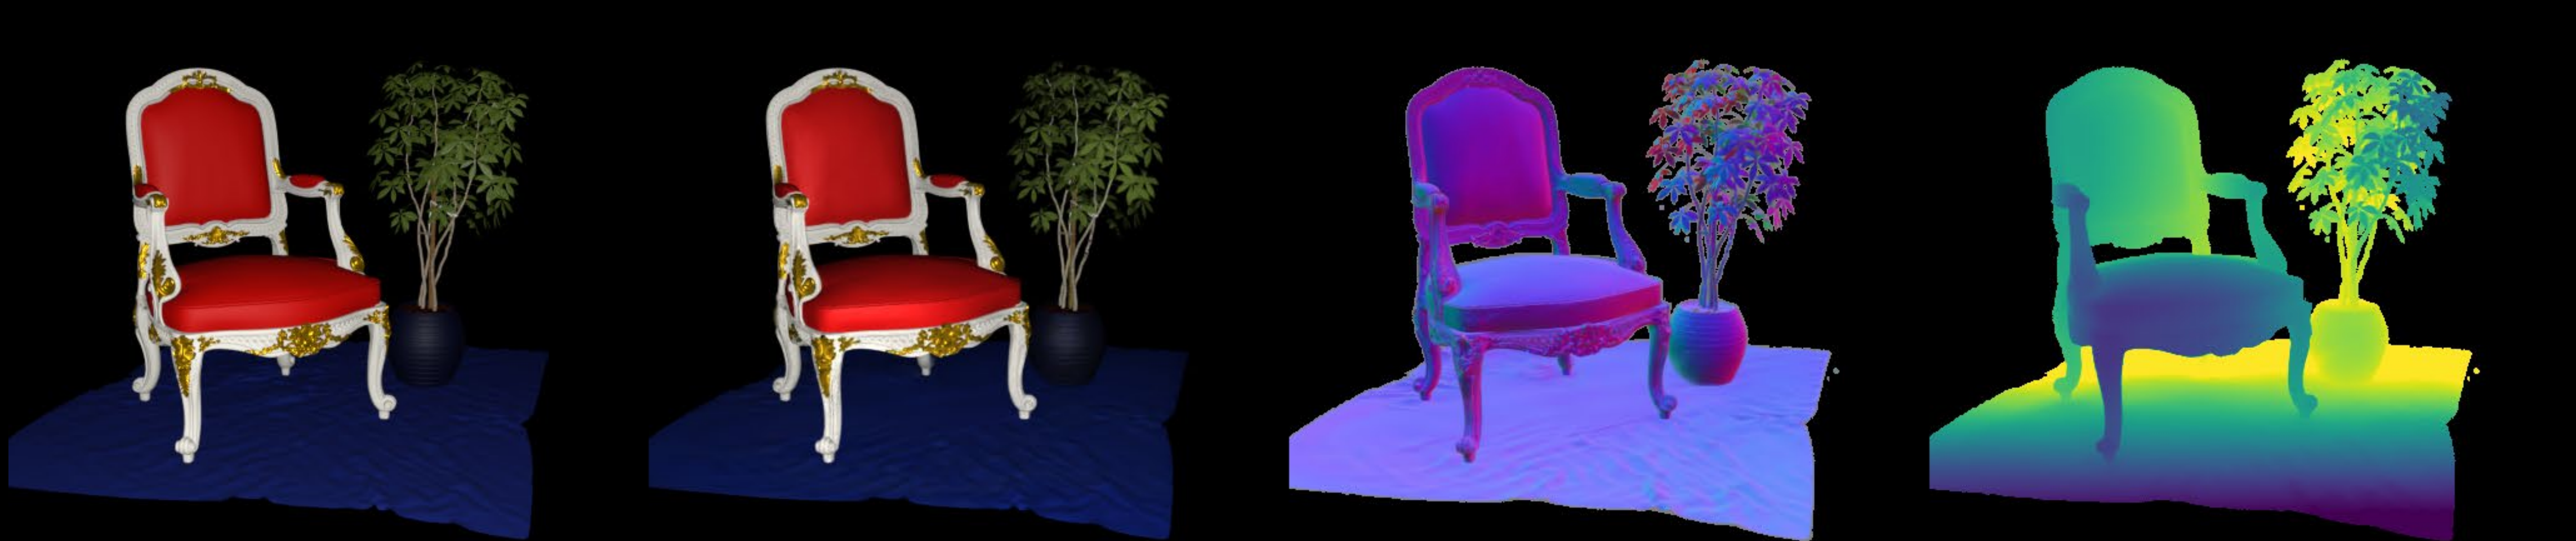

GT

Rendered image

Normal

Depth

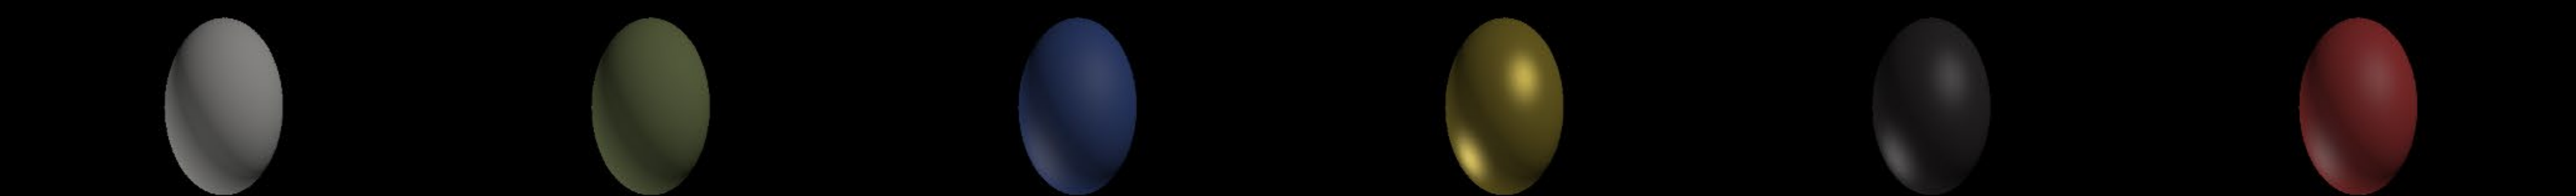

Basis BRDFs

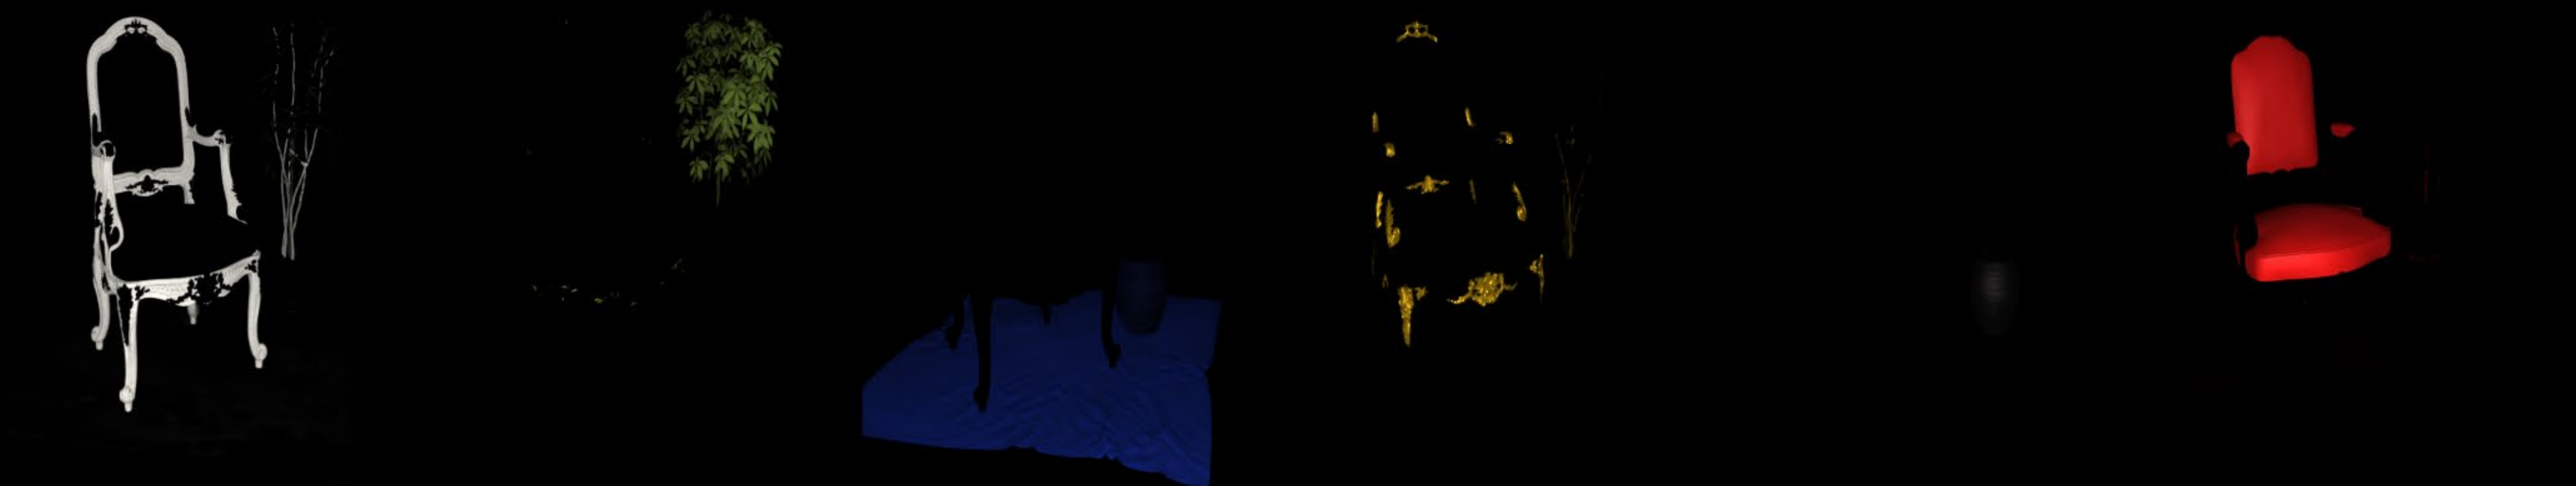

Basis BRDF images

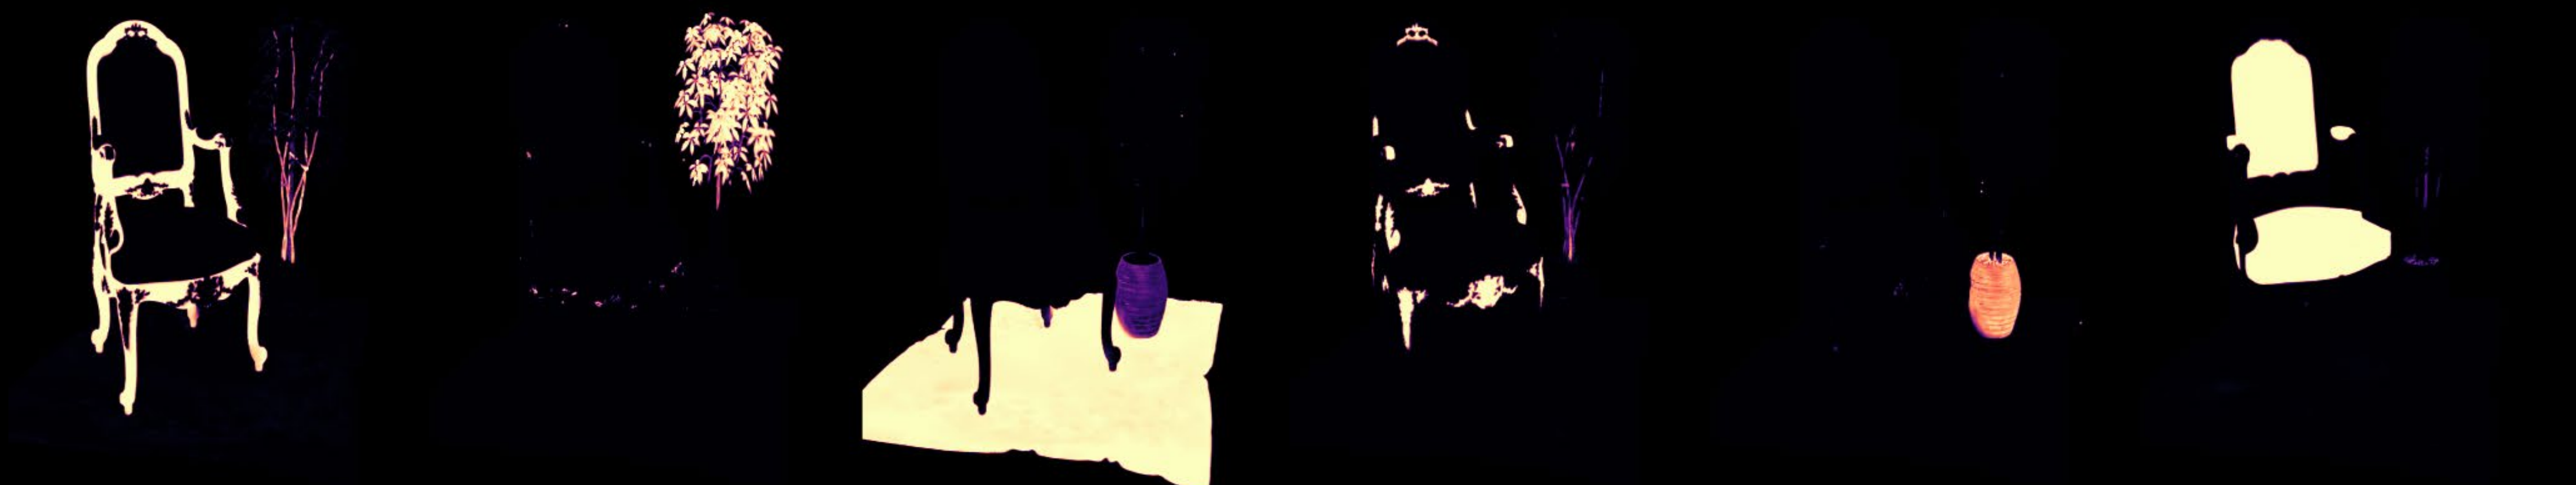

Basis BRDF weight maps



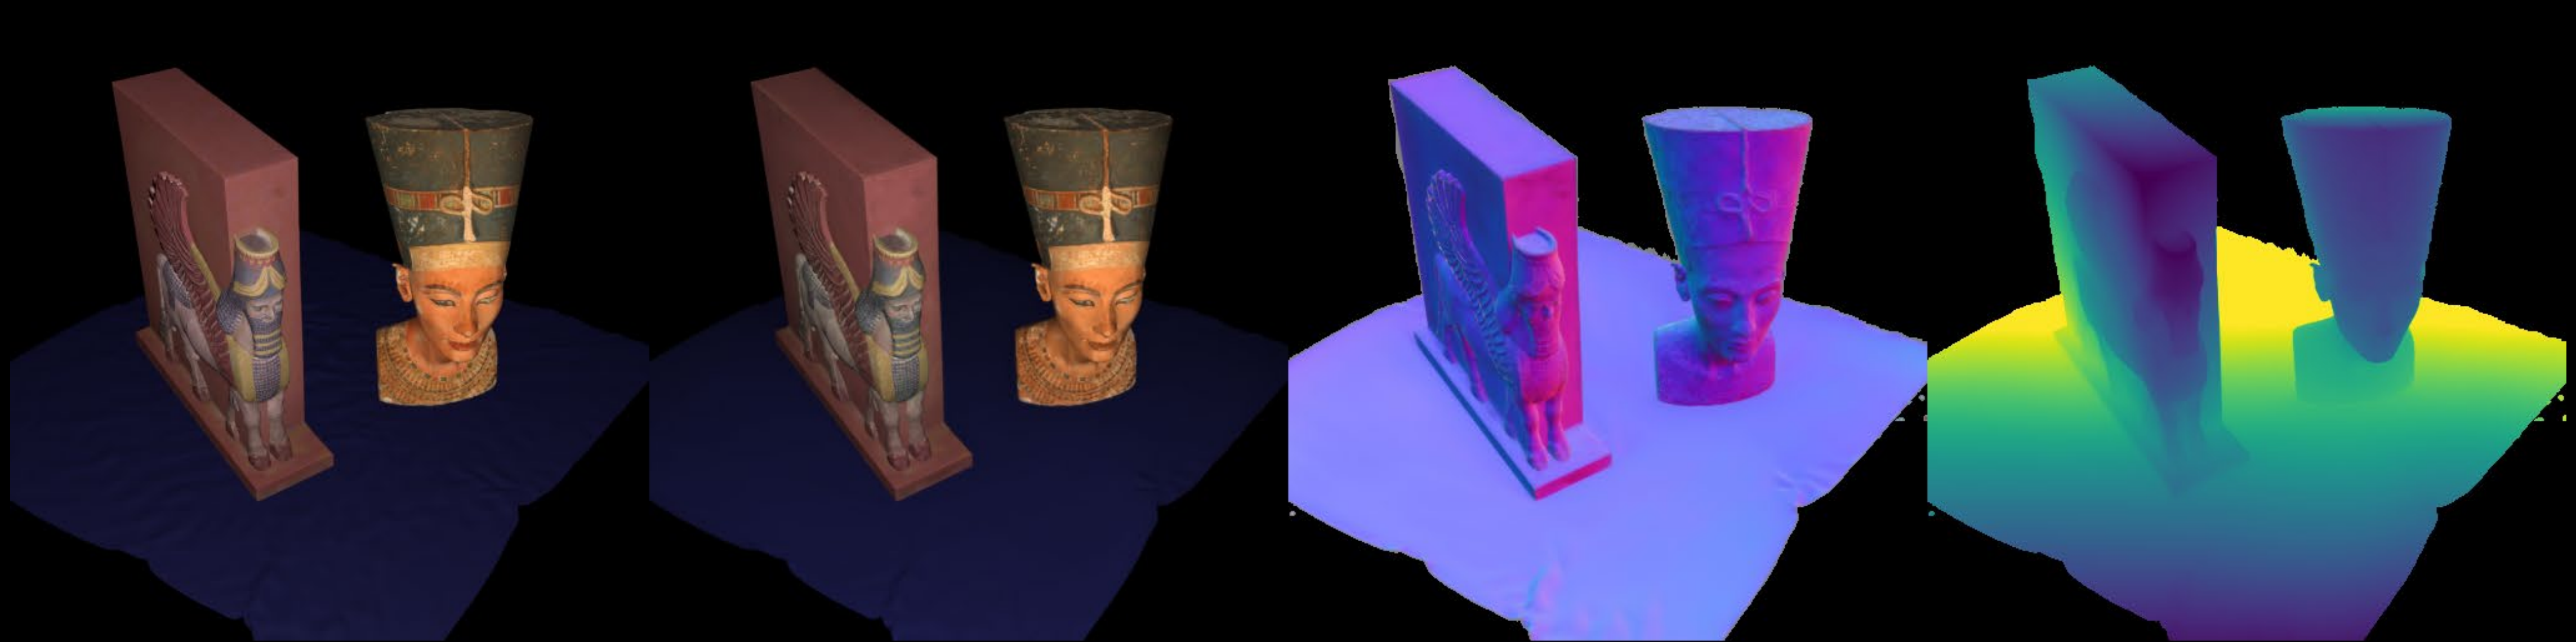

GT

Rendered image

Normal

Depth

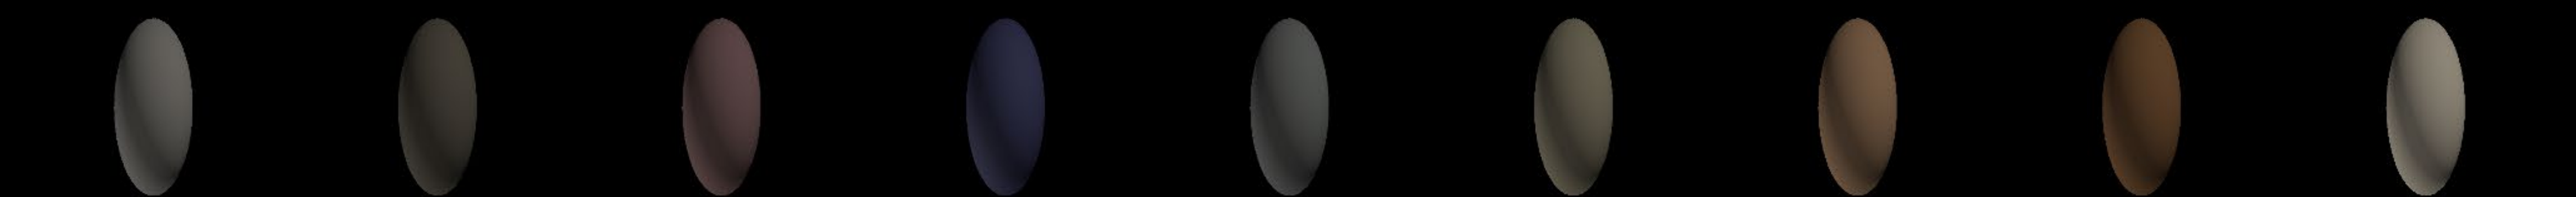

Basis BRDFs

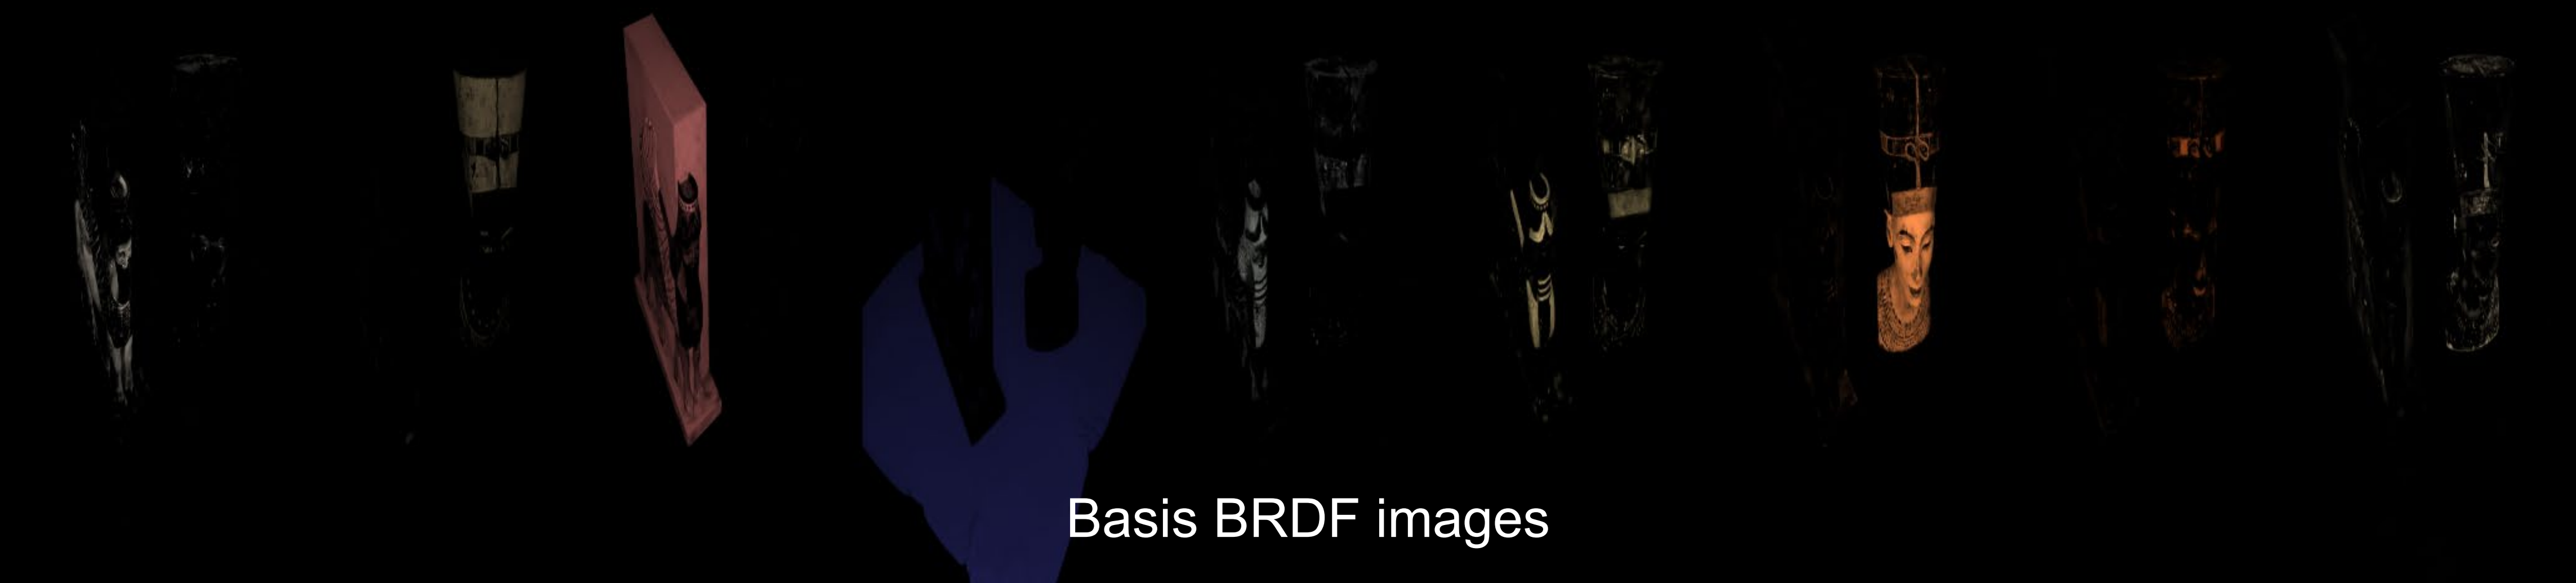

Basis BRDF images

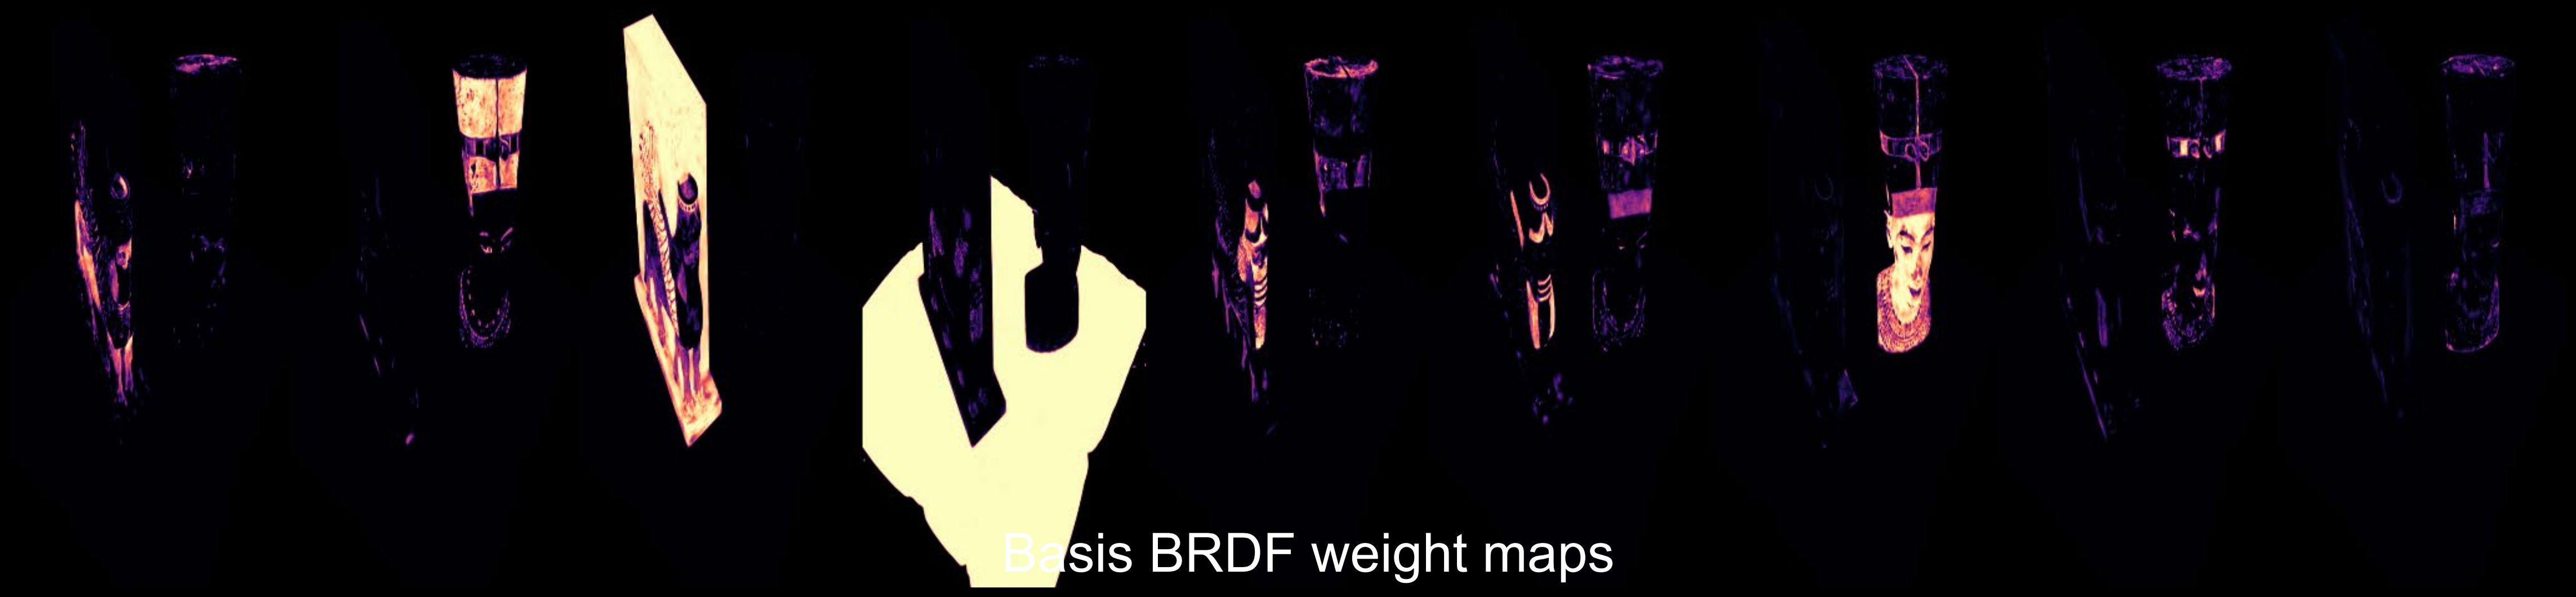

Basis BRDF weight maps
